# Supplementary material for: Revisiting the Formulation of Charged Defect in Solids
Source: arXiv:2407.08504 ancillary file (2024-07-11)
Supplement: Supplementary file 1 [file Supplemental_Materials.pdf]

# Supplemental Materials for Revisiting the Formulation of Charged Defect in Solids

**Hanzhi Shang, Zeyu Jiang, Yiyang Sun, Damien West, and SB Zhang**

**Department of Physics, Applied Physics and Astronomy,**

**Rensselaer Polytechnic Institute, Troy, NY 12180, USA**

1. Electrostatic energy in total energy calculation

Starting from Eq. (3) in the main text,

$$E_0 = \lim_{\boldsymbol{G}\to 0} \Omega \left(\frac{1}{2}V_{coul}(\boldsymbol{G}) + U_{ps}(\boldsymbol{G})\right)\eta(\boldsymbol{G}) + \frac{1}{2}\sum\nolimits_{\nu}' \frac{2Z^2}{|R_\nu|},$$

we need explicit expressions for $V_{coul}(\boldsymbol{G})$, $U_{ps}(\boldsymbol{G})$, and $\eta(\boldsymbol{G})$, as well as the Ewald sum, which we determine by expanding $\eta(\boldsymbol{G})$ to second order.

Calculating the leading terms of electron density in Fourier form yields,

$$\eta(\boldsymbol{G}) = \frac{1}{\Omega}\int_{\Omega} e^{-i\boldsymbol{G}\cdot\boldsymbol{r}}\eta(\boldsymbol{r})d^3r \approx \frac{1}{\Omega}\int_{\Omega}\left(1 - i\boldsymbol{G}\cdot\boldsymbol{r} - \frac{(\boldsymbol{G}\cdot\boldsymbol{r})^2}{2}\right)\eta(\boldsymbol{r})d^3r = \frac{Z_e}{\Omega} + \beta_e G^2. \qquad (S1)$$

The electron potential $V_{Coul}(\boldsymbol{G})$ can then be determined from Poisson' equation,

$$V_{Coul}(\boldsymbol{G}) = 8\pi\,\frac{\eta(\boldsymbol{G})}{G^2} = \frac{8\pi}{G^2}\left(\frac{Z_e}{\Omega} + \beta_e G^2\right) \qquad (S2)$$

Similarly, with the ion density $\eta_I(\boldsymbol{G}) \approx \frac{Z_I}{\Omega} + \beta_I G^2$, the pseudo potential $U_{ps}(\boldsymbol{G})$ becomes.

$$U_{ps}(\boldsymbol{G}) = \frac{8\pi}{G^2}\left(-\frac{Z_I}{\Omega} - \beta_I G^2\right) + \alpha_1. \qquad (S3)$$

The last term in Eq. (3) represents ion-ion interaction,

$$\frac{1}{2}\sum_{\nu,|\boldsymbol{R}_\nu|\neq 0} \frac{2Z^2}{|\boldsymbol{R}_\nu|} = \gamma_{Ewald} + \frac{\Omega}{2}\lim_{G\to 0}\eta_I(G)V_I(G)\,, \qquad (S4)$$

where $\gamma_{Ewald}$ is calculated with the average potential set to zero [10]. Keeping up to second order terms in $\eta_I(\boldsymbol{G}) \approx \frac{Z_I}{\Omega} + \beta_I G^2$, Eq. (S4) becomes,

$$\frac{1}{2}\sum_{\nu,|\boldsymbol{R}_\nu|\neq 0} \frac{2Z^2}{|\boldsymbol{R}_\nu|} = \gamma_{Ewald} + \frac{1}{2}\lim_{G\to 0}\frac{8\pi\Omega}{G^2}\left(\frac{Z_I}{\Omega} + \beta_I G^2\right)^2 \tag{S5}$$

Inserting Eqs. (S1-S5) into Eq. (3), we have

$$E_0 = \lim_{G\to 0}\Omega\left(\frac{1}{2}\frac{8\pi}{G^2}\left(\frac{Z_e}{\Omega} + \beta_e G^2\right)^2 + \left(-\frac{8\pi}{G^2}\left(\frac{Z_I}{\Omega} + \beta_I G^2\right) + \alpha_1\right)\left(\frac{Z_e}{\Omega} + \beta_e G^2\right)\right) + \gamma_{Ewald}$$

$$+ \frac{1}{2}\lim_{G\to 0}\frac{8\pi\Omega}{G^2}\left(\frac{Z_I}{\Omega} + \beta_I G^2\right)^2$$

$$= \gamma_{Ewald} + \alpha_1 Z_e + (Z_e - Z_I)8\pi(\beta_e - \beta_I) + \lim_{G\to 0}\frac{4\pi}{\Omega G^2}(Z_e - Z_I)^2 \tag{S6}$$

According to Eq. (4) of the main text,

$$\bar{V}_e = \lim_{G\to 0} 8\pi\frac{\eta(\boldsymbol{G})}{G^2} = 8\pi\beta_e + \lim_{G\to 0}\frac{8\pi}{G^2}\frac{Z_e}{\Omega}$$

$$\bar{V}_I = -\lim_{G\to 0} 8\pi\frac{\eta_I(\boldsymbol{G})}{G^2} = -8\pi\beta_I - \lim_{G\to 0}\frac{8\pi}{G^2}\frac{Z_I}{\Omega},$$

resulting in, $\bar{V} = \bar{V}_e + \bar{V}_I = 8\pi(\beta_e - \beta_I) + \lim_{G\to 0}\frac{8\pi}{G^2}\frac{Z_e - Z_I}{\Omega}$. Hence the third term in Eq. (S6) can be rewritten as

$$(Z_e - Z_I)8\pi(\beta_e - \beta_I) = (Z_e - Z_I)(\bar{V}_e + \bar{V}_I) \tag{S7}$$

within Eq. (S7), yielding to the final expression of $E_0$ presented as Eq. (5) in the main text,

$$E_0 = \gamma_{Ewald} + \alpha_1 Z_e + (Z_e - Z_I)\bar{V} - \lim_{G\to 0}\frac{4\pi}{G^2}\frac{(Z_e - Z_I)^2}{\Omega}.$$

## 2. Dielectric screening involving localized states of a defect

The electronic screening in a solid can be written as [22]

$$\varepsilon(\hat{q}) \approx 1 + \frac{16\pi}{\Omega} \sum_{nn',\vec{k}} \frac{w_{\vec{k}} \left| \langle \Psi_{n'\vec{k}} | \hat{q} \cdot \vec{r} | \Psi_{n\vec{k}} \rangle \right|^2}{E_{n'\vec{k}} - E_{n\vec{k}}} \tag{S8}$$

where $\hat{q}$ is a unit vector for $\vec{q}$, $n$ and $n'$ refer to the occupied and unoccupied states, and $w_{\vec{k}}$ is a weighting factor. As $\varepsilon$ arises from the sum of transitions, we can separate the defect contribution from that involving only bulk transitions, i.e., $\varepsilon = \varepsilon_{bulk} + \varepsilon_D$. For bulk transitions, the sum over non-vanishing (excluding pseudo-direct transitions from band folding) inter-state transitions $n \to n'$ scales with $\Omega$ and cancels the $^1/_\Omega$ overall factor, reflecting $\varepsilon_{bulk}$ is independent of supercell size. However, for transitions involving the defect, $\left| \langle \Psi^{(i)}_{D\vec{k}} | \hat{q} \cdot \vec{r} | \Psi_{n\vec{k}} \rangle \right|^2 \propto 1/\Omega$ and the number of terms in the sum grow as $\Omega$, yielding an overall volume dependence given in Eq. (17).

3. Evolution of vacancy levels with supercell size

For a vacancy in the tetrahedral structure, we can start with four (degenerate) dangling bond states of energy $e_{DB}$, which interact with each other and hybridize into the localized $a_1$ and $t_2$ states. There will be two types of interactions here, $V_1$ and $V_2$; $V_1$ is within a supercell and is a constant and $V_2$ is between supercells. In the latter case, we assume the dangling bonds, whose separation within a supercell is much smaller than the cell size, are all at the vacancy sites, which allows us to write $V_2 = \lambda/L^2$ and

$$H = \begin{pmatrix} e_{DB} & 0 & 0 & 0 \\ 0 & e_{DB} & 0 & 0 \\ 0 & 0 & e_{DB} & 0 \\ 0 & 0 & 0 & e_{DB} \end{pmatrix} - \begin{pmatrix} 0 & V_1 & V_1 & V_1 \\ V_1 & 0 & V_1 & V_1 \\ V_1 & V_1 & 0 & V_1 \\ V_1 & V_1 & V_1 & 0 \end{pmatrix} - \begin{pmatrix} 0 & V_2 & V_2 & V_2 \\ V_2 & 0 & V_2 & V_2 \\ V_2 & V_2 & 0 & V_2 \\ V_2 & V_2 & V_2 & 0 \end{pmatrix}. \quad (S9)$$

Diagonalization of Eq. (S9) yields

$$H = \begin{pmatrix} e_{DB} - 3V_1 & 0 & 0 & 0 \\ 0 & e_{DB} + V_1 & 0 & 0 \\ 0 & 0 & e_{DB} + V_1 & 0 \\ 0 & 0 & 0 & e_{DB} + V_1 \end{pmatrix} + \begin{pmatrix} -3V_2 & 0 & 0 & 0 \\ 0 & V_2 & 0 & 0 \\ 0 & 0 & V_2 & 0 \\ 0 & 0 & 0 & V_2 \end{pmatrix}. \quad (S10)$$

Defining $e_{a_1}^{L=\infty} = e_{DB} - 3V_1$ and $e_{t_2}^{L=\infty} = e_{DB} + V_1$, one can write the size-dependent energies as follows:

$$\begin{pmatrix} E_{a_1}(L) \\ E_{t_2}(L) \\ E_{t_2}(L) \\ E_{t_2}(L) \end{pmatrix} = \begin{pmatrix} e_{a_1}^{L=\infty} - {}^{3\lambda}/_{L^2} \\ e_{t_2}^{L=\infty} + {}^{\lambda}/_{L^2} \\ e_{t_2}^{L=\infty} + {}^{\lambda}/_{L^2} \\ e_{t_2}^{L=\infty} + {}^{\lambda}/_{L^2} \end{pmatrix} \quad (S11)$$

Eq. (S11) explains the results in Fig. 2(d) where $E_{t_2}(L) - e_{VBM}$ is plotted and found to have $L^{-2}$ dependence.

4. Extension to non-cubic anisotropic supercells

In the defect correction, the localized screened quadrupole in Eq. (16) is determined by subtracting the charge density of screened jellium. To extend this quadrupole correction to the case of non-cubic/anisotropic supercells, the screening of jellium in such supercells must be determined. Here, we start with the screening response due to a point charge $q_p$. From the Green's function [29], the screened electrostatic potential for $q_p$ at origin in an anisotropic dielectric medium is given by

$$V(\boldsymbol{r}) = \frac{1}{\sqrt{det(\bar{\varepsilon})}} \frac{q_p}{\sqrt{\boldsymbol{r^t}\,\bar{\varepsilon}^{-1}\boldsymbol{r}}} \quad (S12)$$

where $\bar{\varepsilon}$ is the dielectric matrix and $\bar{\varepsilon}^{-1}$ is its inverse. Apart from the origin at which $V(\boldsymbol{r})$ diverges, at any other point the electrostatic field $\boldsymbol{E}(\boldsymbol{r})$ can be obtained by taking the gradient of Eq. (S12).

$$\boldsymbol{E}(\boldsymbol{r}) = -\nabla V(\boldsymbol{r}) = -\frac{1}{\sqrt{det(\bar{\varepsilon})}} \nabla \frac{q_p}{\sqrt{\boldsymbol{r^t}\,\bar{\varepsilon}^{-1}\boldsymbol{r}}}$$

$$= -\frac{q_p}{\sqrt{\det(\bar{\varepsilon})}} \nabla \frac{1}{\sqrt{\varepsilon_{11}^{-1}x^2 + \varepsilon_{22}^{-1}y^2 + \varepsilon_{33}^{-1}z^2 + 2\varepsilon_{12}^{-1}xy + 2\varepsilon_{23}^{-1}yz + 2\varepsilon_{13}^{-1}xz}}$$

$$= \frac{q_p}{\sqrt{\det(\bar{\varepsilon})}} \frac{(\varepsilon_{11}^{-1}x + \varepsilon_{12}^{-1}y + \varepsilon_{13}^{-1}z, \varepsilon_{22}^{-1}y + \varepsilon_{12}^{-1}x + \varepsilon_{23}^{-1}z, \varepsilon_{33}^{-1}z + \varepsilon_{13}^{-1}x + \varepsilon_{23}^{-1}y)}{(\varepsilon_{11}^{-1}x^2 + \varepsilon_{22}^{-1}y^2 + \varepsilon_{33}^{-1}z^2 + 2\varepsilon_{12}^{-1}xy + 2\varepsilon_{23}^{-1}yz + 2\varepsilon_{13}^{-1}xz)^{\frac{3}{2}}} \quad (S13)$$

where $\boldsymbol{r} = (x, y, z)$ and $\varepsilon_{ij}^{-1}$ are the components of $\bar{\varepsilon}^{-1}$. Next, we apply Gauss' law in spherical coordinates to obtain the net charge $C(r)$ within the sphere $|\boldsymbol{r}| = r_0$.

$$4\pi C(r_0) = \oiint \boldsymbol{E}(\boldsymbol{r}) \cdot d\boldsymbol{s} = \int_0^{\pi} d\theta \, sin\,\theta \int_0^{2\pi} d\phi \, {r_0}^2 \, \boldsymbol{E}(\boldsymbol{r}) \cdot \frac{\boldsymbol{r}}{r_0}$$

$$= \frac{r_0 q_p}{\sqrt{\det(\bar{\varepsilon})}} \int_0^{\pi} d\theta \, sin\,\theta \frac{(\varepsilon_{11}^{-1}x + \varepsilon_{12}^{-1}y + \varepsilon_{13}^{-1}z, \varepsilon_{22}^{-1}y + \varepsilon_{12}^{-1}x + \varepsilon_{23}^{-1}z, \varepsilon_{33}^{-1}z + \varepsilon_{13}^{-1}x + \varepsilon_{23}^{-1}y)}{(\varepsilon_{11}^{-1}x^2 + \varepsilon_{22}^{-1}y^2 + \varepsilon_{33}^{-1}z^2 + 2\varepsilon_{12}^{-1}xy + 2\varepsilon_{23}^{-1}yz + 2\varepsilon_{13}^{-1}xz)^{\frac{3}{2}}} \cdot (x, y, z)$$

$$= \frac{r_0 q_p}{\sqrt{\det(\bar{\varepsilon})}} \int_0^{\pi} d\theta \, sin\,\theta \int_0^{2\pi} d\phi \frac{\varepsilon_{11}^{-1}x^2 + \varepsilon_{22}^{-1}y^2 + \varepsilon_{33}^{-1}z^2 + 2\varepsilon_{12}^{-1}xy + 2\varepsilon_{23}^{-1}yz + 2\varepsilon_{13}^{-1}xz}{(\varepsilon_{11}^{-1}x^2 + \varepsilon_{22}^{-1}y^2 + \varepsilon_{33}^{-1}z^2 + 2\varepsilon_{12}^{-1}xy + 2\varepsilon_{23}^{-1}yz + 2\varepsilon_{13}^{-1}xz)^{\frac{3}{2}}}$$

$$= \frac{r_0 q_p}{\sqrt{\det(\bar{\varepsilon})}} \int_0^{\pi} d\theta \, sin\,\theta \int_0^{2\pi} d\phi \frac{1}{(\varepsilon_{11}^{-1}x^2 + \varepsilon_{22}^{-1}y^2 + \varepsilon_{33}^{-1}z^2 + 2\varepsilon_{12}^{-1}xy + 2\varepsilon_{23}^{-1}yz + 2\varepsilon_{13}^{-1}xz)^{\frac{1}{2}}}$$

$$= \frac{r_0 q_p}{\sqrt{\det(\bar{\varepsilon})}} \int_0^{\pi} d\theta \, sin\,\theta \int_0^{2\pi} \frac{d\phi}{\sqrt{\hat{\boldsymbol{r}}^{\boldsymbol{t}} \, \bar{\varepsilon}^{-1} \hat{\boldsymbol{r}}}}$$

$$= \frac{C_0}{\sqrt{\det(\bar{\varepsilon})}} \int_0^{\pi} d\theta \, sin\,\theta \int_0^{2\pi} \frac{d\phi}{\sqrt{\hat{\boldsymbol{r}}^{\boldsymbol{t}} \, \bar{\varepsilon}^{-1} \hat{\boldsymbol{r}}}}. \qquad (S14)$$

In the last step we have replace $\boldsymbol{r}$ by $r_0\hat{\boldsymbol{r}}$, thereby eliminating $r_0$ from Eq. (S14). The fact that the net charge $C(r_0)$ is independent of $r_0$ is appealing, as it indicates that the net screening charge in any spherical shell vanishes and due to screening the charge $q_p$ at the origin is reduced to

$$q_{sc} \equiv C(r_0 \to 0) = \frac{q_p}{4\pi\sqrt{\det(\bar{\varepsilon})}} \int_0^{\pi} d\theta \, sin\,\theta \int_0^{2\pi} \frac{d\phi}{\sqrt{\hat{\boldsymbol{r}}^{\boldsymbol{t}} \, \bar{\varepsilon}^{-1} \hat{\boldsymbol{r}}}}. \qquad (S15)$$

More generally, for a bare charge density $\rho_{bare}(\boldsymbol{r}')$, the screened charge density

$$\rho_{sc}(\boldsymbol{r}) = \int d^3r' K(\boldsymbol{r}, \boldsymbol{r}') \rho_{bare}(\boldsymbol{r}'), \qquad (S16)$$

where $K(\boldsymbol{r}, \boldsymbol{r}')$ is the screening kernel. For $q_p$ at the origin ($\boldsymbol{r}' = 0$), the total screened charge in a sphere of radius $r_0$ becomes,

$$q_{sc} = \int_{r \le r_0} d^3r \int d^3r' \, K(\boldsymbol{r}, \boldsymbol{r}') q_p \delta(\boldsymbol{r}') = q_p \int_{r \le r_0} d^3r \, K(\boldsymbol{r}, 0) \qquad (S17)$$

Comparing to Eq. (S15) this yields the following expression,

$$\int_{r\leq r_0} d^3r\, K(\boldsymbol{r},0) = \frac{1}{4\pi\sqrt{\det(\bar{\varepsilon})}}\int_0^{\pi} d\theta\, \sin\theta \int_0^{2\pi} \frac{d\phi}{\sqrt{\hat{\boldsymbol{r}}^{\boldsymbol{t}}\, \bar{\varepsilon}^{-1}\hat{\boldsymbol{r}}}} = \frac{q_{sc}}{q_p}. \qquad (S18)$$

More generally, as the screened charge at $\boldsymbol{r}$ due to a bare charge at $\boldsymbol{r}'$ does not depend on the position of the origin, for a point charge at $\boldsymbol{r}'$ $K(\boldsymbol{r},\boldsymbol{r}')$ can be replaced with $K(\boldsymbol{r}-\boldsymbol{r}')$, yielding

$$\int_{|\boldsymbol{r}-\boldsymbol{r}'|\leq r_0} d^3r\, K(\boldsymbol{r}-\boldsymbol{r}') = \frac{q_{sc}}{q_p}. \qquad (S18')$$

For jellium, the charge density before screening is a uniform $-\frac{q}{\Omega}$ and the screened jellium charge $\rho_{jel,sc}(\boldsymbol{r})$ can be determined from

$$\rho_{jel,sc}(\boldsymbol{r}) = \iiint_{\infty} d^3r'\, K(\boldsymbol{r}-\boldsymbol{r}')\left(-\frac{q}{\Omega}\right) = -\frac{q}{\Omega}\frac{q_{sc}}{q_p} = -\frac{q}{\Omega}\frac{1}{\varepsilon_{eff}}, \qquad (S19)$$

where, we have introduced and effective dielectric constant $\varepsilon_{eff}$, which from Eq. (S18) becomes,

$$\frac{1}{\varepsilon_{eff}} = \frac{1}{4\pi\sqrt{\det(\bar{\varepsilon})}}\int_0^{\pi} d\theta\, \sin\theta \int_0^{2\pi} \frac{d\phi}{\sqrt{\hat{\boldsymbol{r}}^{\boldsymbol{t}}\, \bar{\varepsilon}^{-1}\hat{\boldsymbol{r}}}}. \qquad (S20)$$

In the limit where $\bar{\varepsilon}$ becomes isotropic, Eq. (S20) is reduced to $\frac{1}{\varepsilon_{eff}} = \frac{1}{\varepsilon}$.

We demonstrate the application of this formulation to the anisotropic non-cubic system $\beta$-$Ga_2O_3$ in Fig. S1. The $\beta$-$Ga_2O_3$ unit cell is monoclinic and C2/m and lattice constants are calculated to be a=12.34 Å, b=3.07 Å, and c=5.87 Å. The dielectric matrix associated with bulk was found to be $\begin{pmatrix} 4.02 & 0 & 0.003 \\ 0 & 4.07 & 0 \\ 0.003 & 0 & 4.10 \end{pmatrix}$. K-point sampling was accomplished with a Monkhorst pack mesh in which the number of grid points for each direction was determined by $20\ /L(\text{Å})$. A kinetic energy cutoff of 400 eV was used for the basis using the PBE functional and the self-consistent charge density was determined using a convergence criterion of $10^{-5}$ eV. As Fig. 1 of the main text suggests that interstitials have substantial quadrupole moments, we use the (+1) Li ib-interstitial in $Ga_2O_3$ as a test case, the structure of which is shown in the unit cell in Fig S1

(a). The uncorrected formation energies for a series of supercell shapes/sizes are shown as black open squares in Fig. S1 (b). Red open circles are those with Madelung correction, while filled blue diamonds are those with both Madelung and quadrupole correction. The fully corrected (Madelung+Quadrupole) results are well converged, with even the $1 \times 2 \times 1$ supercell yielding formation energies within 25meV of the dilute limit.

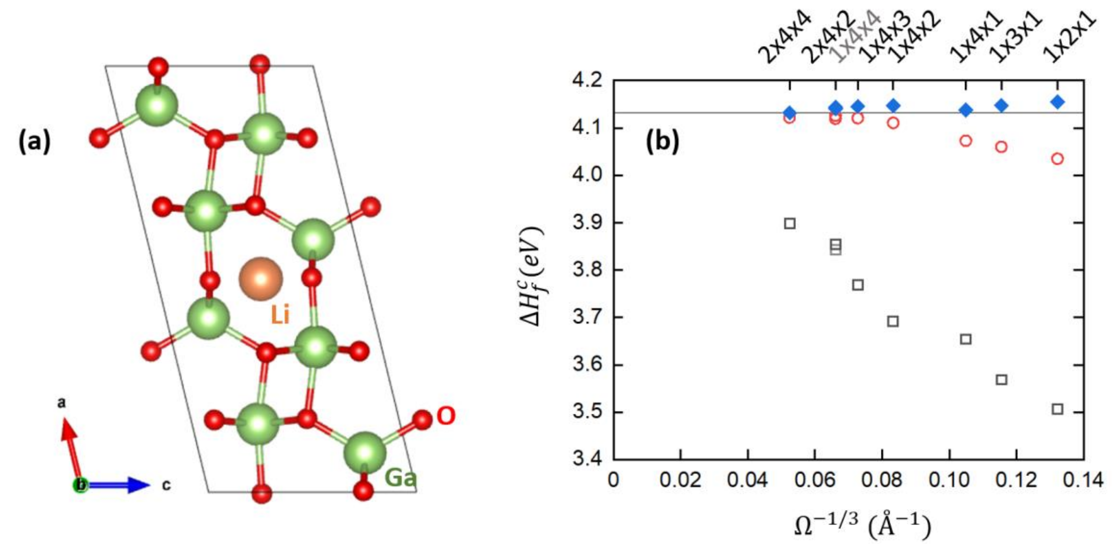


FIG. S1. (a) Atomic structure of $\beta$-$Ga_2O_3$ unit cell and Li interstitial site. (b) Formation energy of Li interstitial in $\beta$-$Ga_2O_3$. Open black squares are raw data. Red open circles are those with Madelung correction, while filled blue diamonds are those with both Madelung and quadrupole correction. Supercell size of the data points is (1) 1x2x1, 1x3x1, 1x4x1 extending $L_y$, (2) 1x4x2, 1x4x3, 1x4x4 extending $L_z$, (3) 2x4x2, 2x4x4 also extending $L_z$, but for larger cell. Note that convergence is dependent on both size and extending direction.
